# Supplementary material for: MolGuidance: Advanced Guidance Strategies for Conditional Molecular Generation with Flow Matching
Source: arXiv:2512.12198 ancillary file (2025-12-13)
Supplement: Supplementary file 1 [file si.pdf]

# Table of contents

**S-1 Mathematical Formulation of Discrete Guidance Formats** **2**

**S-2 Interpolants, Priors and Loss Functions** **2**

**S-3 Model Architecture** **3**

**S-4 Equivariant Optimal Transport** **4**

**S-5 Additional Results** **4**

S-5.1 Different Discrete Guidance Result for 5 Property in QM9 Dataset . . . . . . . . . 4
S-5.2 Hybrid Guidance Result for 5 Property in QM9 Dataset . . . . . . . . . . . . . . . 4
S-5.3 Bayesian optimized guidance weights targeting property alignment. . . . . . . . . 4
S-5.4 Property Alignment . . . . . . . . . . . . . . . . . . . . . . . . . . . . . . . . . 8
S-5.5 Structural Validity . . . . . . . . . . . . . . . . . . . . . . . . . . . . . . . . . 9
S-5.5.1 Molecule stability . . . . . . . . . . . . . . . . . . . . . . . . . . . 9
S-5.5.2 RDKit validity . . . . . . . . . . . . . . . . . . . . . . . . . . . . . 9
S-5.5.3 PoseBusters validity . . . . . . . . . . . . . . . . . . . . . . . . . . 10
S-5.6 Structural Diversity . . . . . . . . . . . . . . . . . . . . . . . . . . . . . . . . 10
S-5.6.1 Bond-order entropy . . . . . . . . . . . . . . . . . . . . . . . . . . . 11
S-5.6.2 Element entropy . . . . . . . . . . . . . . . . . . . . . . . . . . . . 11
S-5.6.3 Scaffold diversity . . . . . . . . . . . . . . . . . . . . . . . . . . . . 11
S-5.7 Training time cost . . . . . . . . . . . . . . . . . . . . . . . . . . . . . . . . . 11
S-5.8 Ablations . . . . . . . . . . . . . . . . . . . . . . . . . . . . . . . . . . . . . 12

**S-6 Original QM9 Properties and Data Details** **14**

# S-1 Mathematical Formulation of Discrete Guidance Formats

**Linear Interpolation (Additive Blend)** Take guidance on probability distribution as an example.

$$p_{\text{guided}} = (1 - w)\, p_{\text{unconditional}} + w\, p_{\text{conditional}} \tag{1}$$

This formula represents a direct, weighted average of the two probability distributions.

**Logarithmic Interpolation (Multiplicative Blend)**

$$\begin{aligned} p_{\text{guided}} &= \exp\left((1 - w)\log p_{\text{unconditional}} + w \log p_{\text{conditional}}\right) &(2)\\ &= \exp\left(\log p_{\text{unconditional}}^{1-w} + \log p_{\text{conditional}}^{w}\right) &(3)\\ &= \exp\left(\log\left(p_{\text{unconditional}}^{1-w} \cdot p_{\text{conditional}}^{w}\right)\right) &(4)\\ &= p_{\text{unconditional}}^{1-w} \cdot p_{\text{conditional}}^{w} &(5)\end{aligned}$$

This is the form operating in log-space, which is mathematically equivalent to a multiplicative blend.

# S-2 Interpolants, Priors and Loss Functions

Flow for atomic positions takes a linear interpolant:

$$X_t = (1 - t)X_0 + tX_1 \tag{6}$$

where $X_0$ and $X_1$ are initial and final states. The base distribution (prior) for atomic positions use a centered standard normal distribution $p_0(X) = \prod_{i=1}^{N} \mathcal{N}(X_0^i|\mathbf{0}, \mathbb{I}_3)$. The optimization of the conditional velocity field for atomic positions can be reparameterized into the optimization of a denoiser network with an mean squared error (MSE) objective:

$$\mathcal{L}_X = \mathbb{E}_{t, p_t(X_t|X_0, X_1), \pi(X_0, X_1)} \left[ \|X_{1|t}^{\theta} - X_1\| \right] \tag{7}$$

Where the joint distribution $\pi(X_0, X_1)$ defines the optimal transport coupling between $(X_0, X_1)$. $X_{1|t}^{\theta}$ represents the predicted atomic position given the state at time $t$. Details of the optimal transport formulation are provided in section S-4.

Discrete variables such as atom types and charges are modeled through the CTMC flows [1]. The prior distribution is the state in which all atoms are in a masked state, and the generation process is essentially a demasking process. We refer the readers to the FlowMol work for more details of the CTMC flows [2]. The objective for these discrete variables takes the cross-entropy format:

$$\mathcal{L}_{\text{CE}} = \mathbb{E}_{t, p_{t|1}(x_t|z), p_z} \left[ -\log p_{1|t}^{\theta}(x_1^i|x_t) \right] \tag{8}$$

The total loss for the molecule graph is a weighted linear summation of losses for each molecular modality:

$$\mathcal{L} = \eta_X \mathcal{L}_X + \eta_A \mathcal{L}_A + \eta_C \mathcal{L}_C + \eta_E \mathcal{L}_E \tag{9}$$

Empirically, it is preferential to determin atomic positions first, followed by bonds, charges and atom types. In view of this, the loss weights are chosen to be $(\eta_X, \eta_A, \eta_C, \eta_E) = (3.0, 0.4, 1.0, 2.0)$.

# S-3 Model Architecture

The vanilla PropMolFlow model uses the 'Concatenate_Sum' property embedding method without a Gaussian expansion, as implemented in our previous work [3]. The backbone model for SE(3)-equivariant joint flow matching adopts the architecture implemented in FlowMol [4]. Molecule updates are achieved through layers comprising of Geometric Vector Perceptrons (GVPs). Within each GVP, the molecule graph passes through a sequential steps of Node Feature Update (NFU), Node Position Update (NPU) and Edge Feature Update (EFU). Each node $i$ consists of a position $x_i \in \mathbb{R}^3$, scalar features $s_i \in \mathbb{R}^d$, and vector features $v_i \in \mathbb{R}^{c\times 3}$. Non-zero vector features are involved a cross-product vector operation, which is crucial to break the reflection symmetry, making it an SE(3) equivariant architecture. The scalar feature is a concatenation of atom type and charge vectors; that is, $s_i = [a_i \oplus c_i]$ where '$\oplus$' defines a concatenation operation. Each edge feature corresponds to the bond order, and the permutation invariance of bond orders is realized through taking the sum of bond features from $i \to j$ and $j \to i$;that is, $\widehat{e}^{ij} = \mathrm{MLP}(e_{ij} + e_{ji})$.

**Node Feature Update.** The node feature takes two steps for its update: the first step generates scalar messages $m^{(s)}_{i\to j}$, and vector messages $m^{(v)}_{i\to j}$ by a function $\psi_M$ which corresponds to a sequential two GVPs:

$$m^{(s)}_{i\to j}, m^{(v)}_{i\to j} = \psi_M\left(\left[s_i^{(l)} \oplus e_{ij}^{(l)} \oplus d_{ij}^{(l)}\right], \left[v_i \oplus \frac{x_i^{(l)} - x_j^{(l)}}{d_{ij}^{(l)}}\right]\right) \tag{10}$$

Where $d_{ij}^{(l)}$ is the distance between nodes $i$ and $j$ at the update layer $l$. To enrich the neighboring environment, the distance $d_{ij}$ is expanded with a radial basis function (RBF) embedding before fed into the next GVPs or MLPs. A message passing procedure is conducted to update node scalar and vector features by aggregation:

$$s_i^{(l+1)}, v_i^{(l+1)} = \mathrm{LN}\left([s_i^{(l)}, v_i^{(l)}] + \psi_N\left(\frac{1}{|\mathcal{N}(i)|}\sum_{j\in\mathcal{N}(i)}\right)\left[m^{(s)}_{j\to i}, m^{(v)}_{j\to i}\right]\right) \tag{11}$$

Where $LN$ stands for s LayerNormalization operation [5], $\psi_N$ is a chain of three GVPs.

**Node Position Update.** Node-wise operations are used on the updated node scalar and vector features to update node position features:

$$x_i^{(l+1)} = x_i^{(l)} + \psi_P\left(s_i^{(l+1)}, v_i^{(l+1)}\right) \tag{12}$$

Where $\psi_P$ is a sequencial three GVPs in which the final output has 1 vector and 0 scalar features.

**Edge Feature Update.** Edge features are updated by edge-wise operations that takes the updated node scalar features and node distance as the inputs:

$$e_{ij}^{(l+1)} = \mathrm{LayerNorm}\left(e_{ij}^{(l)} + \mathrm{MLP}\left(s_i^{(l+1)}, s_j^{(l+1)}, d_{ij}^{(l+1)}\right)\right) \tag{13}$$

# S-4 Equivariant Optimal Transport

To smooth the probability path, we used the equivariant optimal transport to align the initially sampled noisy molecules with the target molecules, as used in previous works [6–8]. This is achieved by optimal permutation of atom node indices and rigid body alignment between base molecules and target molecules, for both of which their center-of-masses are removed to respect the translational invariance [8, 9].

# S-5 Additional Results

## S-5.1 Different Discrete Guidance Result for 5 Property in QM9 Dataset

Result is shown in Figure S1.

## S-5.2 Hybrid Guidance Result for 5 Property in QM9 Dataset

Result is shown in Figure S2.

## S-5.3 Bayesian optimized guidance weights targeting property alignment.

Figure S3 illustrates a schematic example of Bayesian optimization (a), the results for CFG weights optimized over the HOMO property (b), AG weights optimized over heat capacity (c), and MG single weight optimized over HOMO-LUMO gaps (d).

MAEs for the MG models vary in a smaller range, suggesting the difficulty in leveraging the guidance weight effects for MG. Also, there are high fluctuations for MAE when guidance weights changes from around 1.6 to 1.7, indicating the instability of the MG model for describing the guidance weight effect.

**Table S1:** Bayesian optimized guidance weights $(w_1, w_2)$ for each method in two datasets. For MG, identical weights apply to both positional and discrete variables. All weights are dimensionless.

| Property | $\alpha$ | $\Delta\epsilon$ | $\epsilon_{\text{HOMO}}$ | $\epsilon_{\text{LUMO}}$ | $\mu$-QM9 | $C_v$ | $\mu$-QMe14S |
|---|---|---|---|---|---|---|---|
| PMF-CFG | (4.00, 1.77) | (4.00, 2.16) | (2.71, 1.91) | (3.97, 2.29) | (4.00, 2.31) | (4.00, 2.00) | (3.13, 1.88) |
| PMF-AG | (2.34, 1.00) | (4.26, 1.34) | (2.79, 1.11) | (3.15, 1.17) | (4.29, 1.50) | (2.75, 1.14) | (2.71, 1.11) |
| PMF-MG | 1.34 | 1.68 | 1.89 | 2.23 | 2.21 | 2.14 | 2.25 |

It is crucial to identify the optimal guidance as the MAEs can vary by more than ten times in certain situations (e.g., from 1.40 to 15.5 Bohr$^3$ for AG conditioned on $\alpha$). The guide model that yields the best performance under AG is provided in Table S3. As a general rule, greater differences between the guide and main models tend to produce lower property MAEs. One may argue that expanding the search range can further improvement the property alignment, since many optimal atomic-position weights $(w_1)$ lie at the boundaries of the search range for both CFG and AG (Table S1). Nevertheless, given the weaker MAE dependence on $w_1$, the additional gain by extending the search space may not be worthwhile. All subsequent performance metrics are computed using models with their corresponding best guidance weights.

Ranges of MAEs for Bayesian optimization can be found in Table S2.

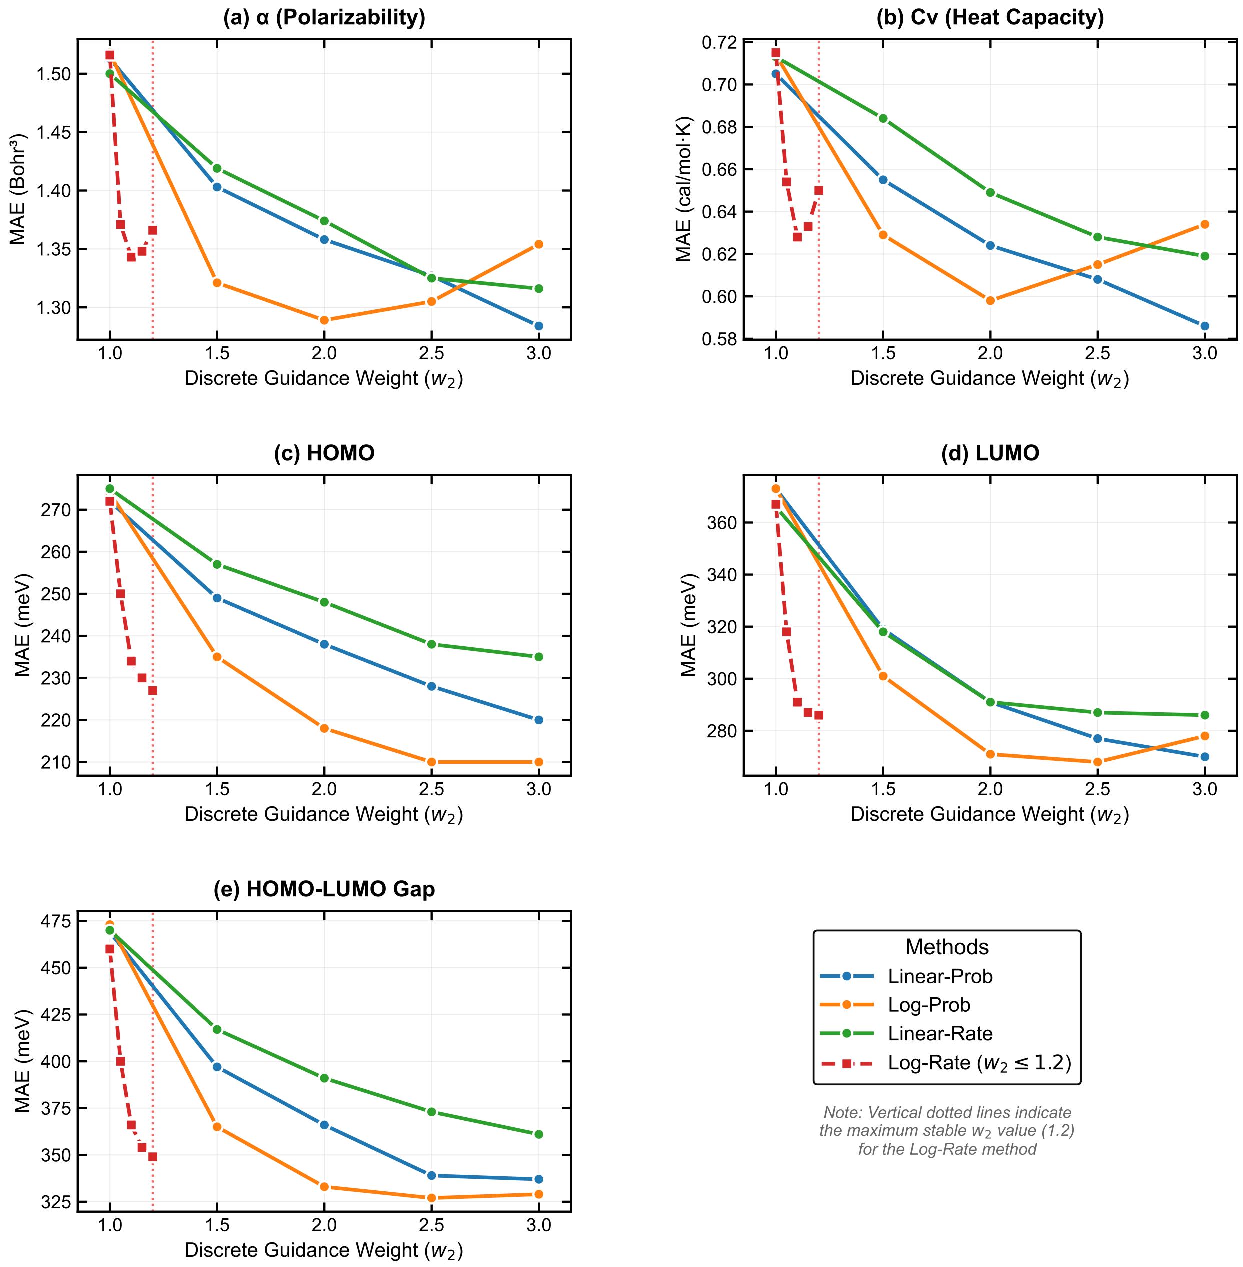


**Figure S1:** Comparison of discrete guidance formats for qm9 dataset across 5 properties. Four guidance methods are compared: linear guidance on probability (Linear-Prob), logarithm guidance on probability (Log-Prob), linear guidance on rate matrix (Linear-Rate) , and logarithm guidance on rate matrix (Log-Rate). The Log-Rate method is constrained to $w_2 \leq 1.2$ due to numerical instability at higher guidance weights, indicated by the vertical dotted line. Lower MAE values indicate better performance.

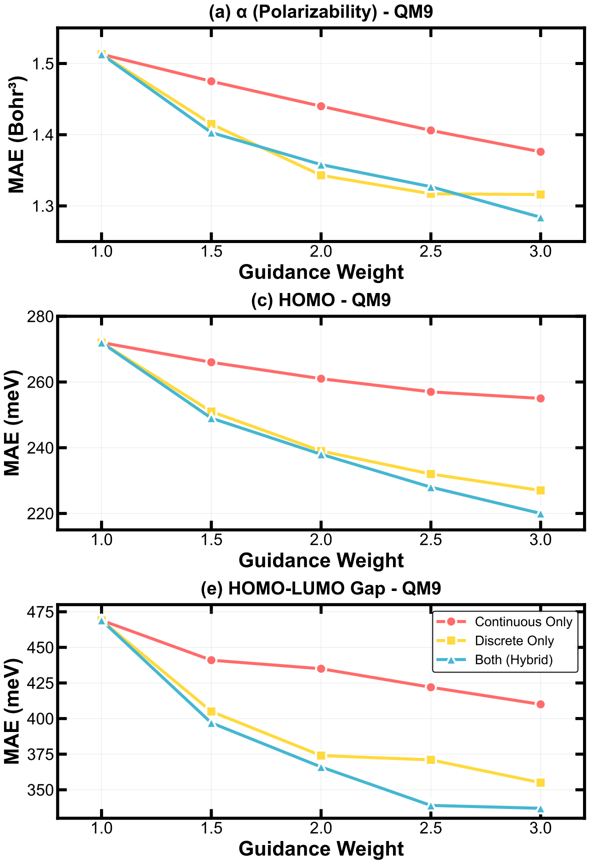


**Figure S2:** MAE for 5 properties alignment using three guidance strategies: continuous-only (atomic positions), discrete-only (atom types, charges, bonds), and hybrid (both domains) on QM9 datasets. Lower MAE values indicate better alignment between target and generated molecule properties

**Table S2:** Ranges of MAEs for Bayesian optimization for different guidance methods. Results are evaluated on 1000 sampled molecules. AG uses the guide model trained with 40000 steps and reduced numbers of node and edge features.

| Property<br>Units | $\alpha$<br>Bohr$^3$ | $\Delta\epsilon$<br>meV | $\epsilon_{\text{HOMO}}$<br>meV | $\epsilon_{\text{LUMO}}$<br>meV | $\mu$-QM9<br>Debye | $C_v$<br>cal/(mol·K) | $\mu$-QMe14S |
|---|---|---|---|---|---|---|---|
| CFG, Minimum MAE | 1.20 | 317 | 202 | 249 | 0.549 | 0.556 | 0.508 |
| CFG, Maximum MAE | 2.68 | 603 | 282 | 757 | 0.746 | 1.684 | 0.708 |
| AG, Minimum MAE | 1.40 | 328 | 231 | 256 | 0.591 | 0.616 | 0.560 |
| AG, Maximum MAE | 15.5 | 425 | 360 | 466 | 0.926 | 1.023 | 0.679 |
| MG, Minimum MAE | 1.53 | 406 | 261 | 333 | 0.714 | 0.689 | 0.628 |
| MG, Maximum MAE | 1.67 | 457 | 280 | 358 | 0.778 | 0.759 | 0.704 |

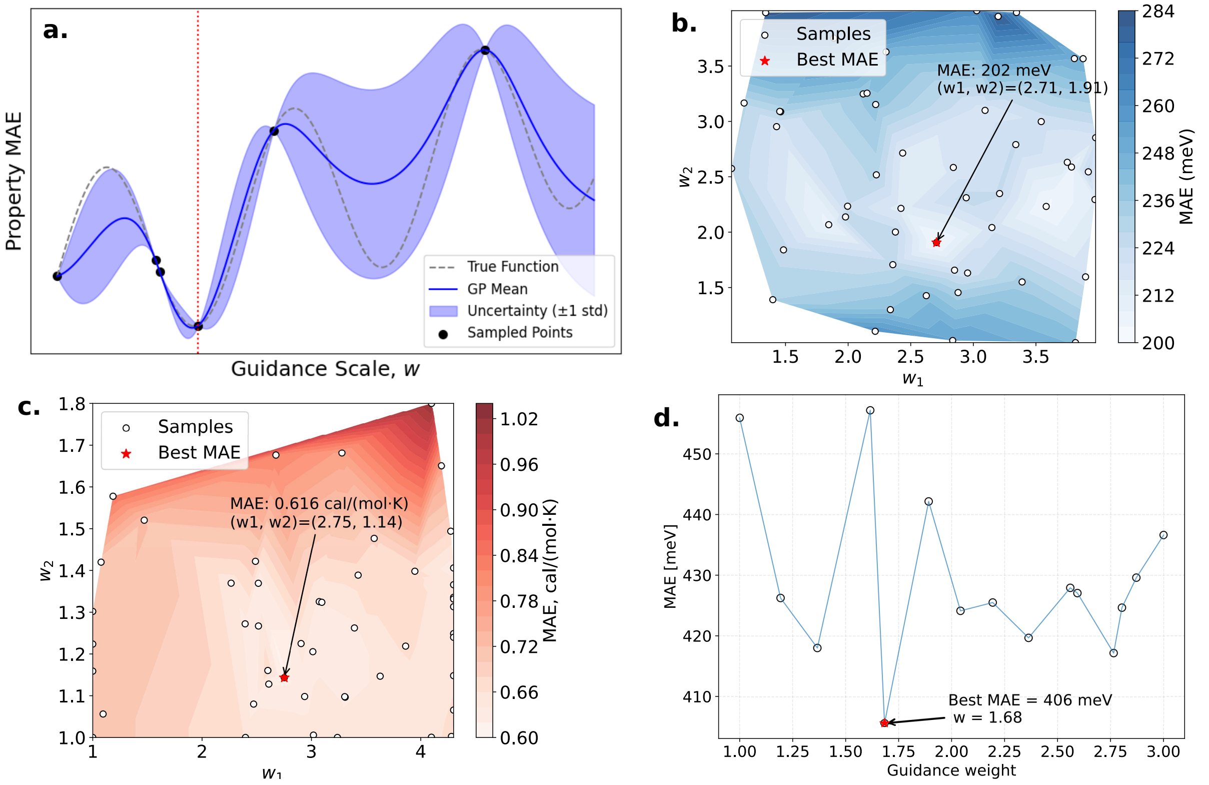


**Figure S3:** Bayesian optimization of guidance weights for property alignment. (a) A 1-D schematic plot of the Bayesian optimization aiming to minimize the property MAEs. (b) Performance of Bayesian optimization over guidance weights for CFG conditioning on HOMO energy. (c) Bayesian optimization over guidance weights for AG conditioning on heat capacity. (d) Bayesian optimization over single guidance weights for MG conditioning on HOMO-LUMO gap values. Hollow circles denote sampled weight pairs, with the best candidate (lowest MAE) highlighted by a red star; its guidance weights and MAE are indicated. MAEs were computed over 1000 molecules sampled from the joint distribution of atom count and property values.

**Comparing performance of two guide models in AG.** The best guide model for each property is summarized in Table S3. The first guide model ($u_{g,1}$) is trained with 40000 steps and has a reduced-by-half numbers of hidden node features and edge features, and the second guide mode ($u_{g,2}$) is the same architecture of the main model but trained with only 51 epochs.

**Table S3:** Bayesian optimized guidance weights and the best MAEs for two different guide models in AG for the QM9 data. Numbers in bracket correspond to $(w_1, w_2)$, which are dimensionless, and values after the weights are corresponding best MAEs. This evaluation is based on 1000 sampled molecules, and the model chosen for further analysis in the main text are **bold**.

| Property<br>Units | $\alpha$<br>Bohr$^3$ | $\Delta\epsilon$<br>meV | $\epsilon_{\mathrm{HOMO}}$<br>meV | $\epsilon_{\mathrm{LUMO}}$<br>meV | $\mu$<br>Debye | $C_v$<br>cal/(mol·K) |
|---|---|---|---|---|---|---|
| $u_{g,1}$ | (2.09, 1.21), 1.40 | **(4.26, 1.34), 328** | **(2.79, 1.11), 231** | **(3.15, 1.17), 256** | **(4.29, 1.50), 0.591** | **(2.75, 1.14), 0.616** |
| $u_{g,2}$ | **(2.34, 1.00), 1.39** | (2.47, 1.42), 330 | (1.93, 1.28), 234 | (3.63, 1.15), 272 | (4.29, 1.20), 0.631 | (1.00, 1.35), 0.672 |

## S-5.4 Property Alignment

Full results of Property MAEs for six different properties and for the QMe14S data conditioned on dipole moment ($\mu$) are shown in Table S4. The "Random" corresponds to MAEs between original molecular properties and fully shuffled properties, removing any correlations between structures and properties, hence serving as an upper bound. The "# Atoms" baseline uses atom counts as the predictor for molecular properties. The "QM9" baseline uses a separate predictor trained on a disjoint 50k molecules to predict properties of the 50k molecules used to train the generative model. The property predictor is trained on the QM9 xyz data [10], and provided by Hoogeboom *et al.* [9], and the corresponding MAE serves as a lower bound on achievable error. Improvement over the "# Atoms" baseline suggests that the generative model captures structural features beyond simple atom count when generating new molecules.

**Table S4:** Mean Absolute Error for molecular property prediction (lower is better). PropMolFlow (PMF) results employ Bayesian-optimized guidance weights. Top-ranked values are **bold**, second-best values are underlined. JODO results are from our own sampled molecules. '/' indicates that the results are unavailable.

| Property<br>Units | $\alpha$<br>Bohr$^3$ | $\Delta\epsilon$<br>meV | $\epsilon_{\mathrm{HOMO}}$<br>meV | $\epsilon_{\mathrm{LUMO}}$<br>meV | $C_v$<br>cal/(mol·K) | $\mu$-QM9<br>Debye | $\mu$-QMe14S<br>Debye |
|---|---|---|---|---|---|---|---|
| QM9 (Lower-Bound) | 0.10 | 64 | 39 | 36 | 0.040 | 0.043 | / |
| Random (Upper-Bound) | 9.01 | 1470 | 645 | 1457 | 6.857 | 1.616 | / |
| # Atoms | 3.86 | 866 | 426 | 813 | 1.971 | 1.053 | / |
| GeoLDM | 2.37 | 587 | 340 | 522 | 1.025 | 1.108 | / |
| GCDM | 1.97 | 602 | 344 | 479 | 0.689 | 0.844 | / |
| JODO | 1.44 | 333 | 231 | **260** | **0.580** | 0.620 | / |
| PMF-Vanilla | 1.49 | 390 | 266 | 325 | 0.702 | 0.667 | 0.627 |
| PMF-CFG | **1.27** | **322** | **220** | 265 | 0.581 | **0.580** | **0.548** |
| PMF-AG | 1.43 | 344 | 242 | 274 | 0.638 | 0.631 | 0.587 |
| PMF-MG | 1.59 | 425 | 273 | 346 | 0.708 | 0.753 | 0.631 |

DFT confirms the property alignment predicted by a GVP property predictor on 500 molecules selected out of 10K generated molecules (Table S5).

**Table S5:** Performance of property alignment for CFG, evaluated using both DFT and a property predictor (GVP). Metrics are computed on 500 molecules selected from the 10k generated molecules reported in Table S4, using the same property units. The 500 molecules were further filtered by molecule stability, closed-shell valence electron configuration, RDKit validity, PoseBusters validity, and DFT convergence.

| Property | $\alpha$ | $\Delta\epsilon$ | $\epsilon_{\text{HOMO}}$ | $\epsilon_{\text{LUMO}}$ | $C_v$ | $\mu$-QM9 | $\mu$-QMe14S |
|---|---|---|---|---|---|---|---|
| DFT vs Target | 1.18 | 341 | 261 | 242 | 0.563 | 0.586 | 0.584 |
| GVP vs Target | 1.21 | 293 | 213 | 225 | 0.528 | 0.580 | 0.557 |

## S-5.5 Structural Validity

### S-5.5.1 Molecule stability

Table S6 shows the molecule stability of generated molecules conditioning on six properties for baseline models and different guidance methods.

**Table S6:** Performance of molecule stability (%). Higher numbers indicate better performance. All results for baseline models are from the PropMolFlow work [3]. The best results are in **bold** and the second best results are underlined.

| Property | $\alpha$ | $\Delta\epsilon$ | $\epsilon_{\text{HOMO}}$ | $\epsilon_{\text{LUMO}}$ | $C_v$ | $\mu$-QM9 | $\mu$-QMe14S |
|---|---|---|---|---|---|---|---|
| GeoLDM | 81.4 | 83.1 | 84.0 | 84.0 | 81.3 | 85.5 | / |
| GCDM | 85.0 | 86.0 | 88.3 | 84.7 | 85.1 | 86.3 | / |
| JODO | 92.7 | 94.1 | 93.5 | 92.5 | 91.7 | 93.7 | / |
| **PMF** | | | | | | | |
| Vanilla | 92.8 | 94.6 | 95.1 | <u>94.2</u> | 91.8 | 96.2 | <u>97.8</u> |
| CFG | 93.1 | 92.5 | 95.6 | 92.0 | 88.4 | 92.8 | 96.8 |
| AG | **95.8** | <u>95.7</u> | **97.2** | **96.9** | **93.9** | <u>96.6</u> | 97.5 |
| MG | <u>94.8</u> | **96.9** | <u>96.9</u> | 93.3 | <u>91.9</u> | **96.8** | **97.9** |

### S-5.5.2 RDKit validity

Table S7 shows the RDKit validity of generated molecules conditioning on six properties for baseline models and different guidance methods.

**Table S7:** RDKit validity (%) for generated molecules conditioned on six properties. All results for baseline models are from the PropMolFlow work [3]. The best results are in **bond** and the second best results are underlined.

| Property | $\alpha$ | $\Delta\epsilon$ | $\epsilon_{\text{HOMO}}$ | $\epsilon_{\text{LUMO}}$ | $\mu$-QM9 | $C_v$ | $\mu$-QMe14S |
|---|---|---|---|---|---|---|---|
| GeoLDM | 91.6 | 91.8 | 92.2 | 92.2 | 93.0 | 89.6 | / |
| GCDM | 94.4 | 94.7 | 95.4 | 94.4 | 94.9 | 94.4 | / |
| JODO | 96.4 | 97.0 | 95.9 | 95.6 | 96.4 | 95.6 | / |
| **PMF** | | | | | | | |
| Vanilla | <u>97.6</u> | **98.4** | 98.3 | <u>97.8</u> | **98.7** | <u>97.0</u> | <u>99.5</u> |
| CFG | 96.8 | 97.4 | 97.9 | 96.6 | 96.5 | 94.0 | 99.0 |
| AG | **98.2** | 97.3 | <u>98.5</u> | **98.0** | 98.0 | **97.6** | **99.6** |
| MG | <u>97.6</u> | <u>98.2</u> | **98.9** | 96.3 | <u>98.6</u> | 96.8 | 99.4 |

### S-5.5.3 PoseBusters validity

Table S8 shows the PoseBusters validity of generated molecules conditioning on six properties for baseline models and different guidance methods.

**Table S8:** PoseBusters validity (%) for generated molecules conditioned on six properties. All results for baseline models are from the PropMolFlow work [3]. The best results are in **bond** and the second best results are underlined.

| Property | $\alpha$ | $\Delta\epsilon$ | $\epsilon_{\mathrm{HOMO}}$ | $\epsilon_{\mathrm{LUMO}}$ | $\mu$-QM9 | $C_v$ | $\mu$-QMe14S |
|---|---|---|---|---|---|---|---|
| GeoLDM | 89.1 | 89.2 | 90.3 | 89.9 | 90.3 | 87.3 | / |
| GCDM | 91.6 | 92.0 | 92.9 | 92.0 | 92.4 | 91.4 | / |
| JODO | 95.2 | 95.7 | 94.7 | 94.5 | 95.3 | 94.1 | / |
| **PMF** | | | | | | | |
| Vanilla | 95.7 | **97.3** | 96.6 | 96.5 | 97.1 | 95.5 | **99.0** |
| CFG | 95.4 | 95.3 | 96.5 | 94.1 | 92.9 | 90.7 | 96.2 |
| AG | **96.7** | 94.6 | 97.3 | **97.5** | 94.0 | **96.2** | 98.4 |
| MG | 95.9 | 97.1 | **97.5** | 95.2 | **97.5** | 95.5 | 98.9 |

## S-5.6 Structural Diversity

Table S9 shows that percentages of molecules that are RDKit valid and unique in their SMILES representation.

**Table S9:** Ratios of unique RDKit valid molecules ('Uniqueness') across different guidance methods. All values are reported in unit of '%', and higher numbers indicate higher structural diversity. The highest values are in **bold**, and the second highest values are underlined.

| Property | $\alpha$ | $\Delta\epsilon$ | $\epsilon_{\mathrm{HOMO}}$ | $\epsilon_{\mathrm{LUMO}}$ | $C_v$ | $\mu$-QM9 | $\mu$-QMe14S |
|---|---|---|---|---|---|---|---|
| Vanilla | **96.0** | **96.6** | 96.5 | **95.6** | **95.6** | **96.5** | 97.8 |
| CFG | 94.3 | 95.3 | 95.4 | 94.5 | 92.3 | 95.0 | 96.8 |
| AG | 95.7 | 93.5 | 95.6 | 94.8 | 95.2 | 94.7 | 97.5 |
| MG | 95.9 | 96.2 | **96.6** | 95.0 | **95.6** | 96.4 | **97.9** |

Table S10 shows that all guidance methods increase bond entropy for most properties compared to the vanilla models. Among guidance approaches, CFG achieves the highest bond entropy for $\Delta\epsilon$, $\epsilon_{\mathrm{HOMO}}$ and $\mu$, whereas AG has the highest bond entropy for $\alpha$ and $C_v$. This elevated bond entropy under CFG and AG can likely be attributed to its relatively high guidance weights on atomic positions (Table S1).

#### S-5.6.1 Bond-order entropy

**Table S10:** Bond-order entropy of generated molecules under various guidance methods. The highest values are in **bold**, and the second highest values are underlined.

| Property | $\alpha$ | $\Delta\epsilon$ | $\epsilon_{\mathrm{HOMO}}$ | $\epsilon_{\mathrm{LUMO}}$ | $\mu$-QM9 | $C_v$ | $\mu$-QMe14S |
|---|---|---|---|---|---|---|---|
| Vanilla | 0.593 | 0.560 | 0.543 | 0.495 | 0.480 | 0.490 | 0.457 |
| CFG | **0.65** | 0.569 | 0.532 | 0.562 | 0.536 | **0.617** | 0.503 |
| AG | 0.599 | **0.657** | **0.598** | 0.556 | **0.556** | 0.498 | **0.598** |
| MG | 0.524 | 0.570 | 0.578 | **0.567** | 0.463 | 0.510 | 0.433 |

#### S-5.6.2 Element entropy

**Table S11:** Element entropy of generated molecules under various guidance methods. The highest values are in **bold**, and the second highest values are underlined.

| Property | $\alpha$ | $\Delta\epsilon$ | $\epsilon_{\mathrm{HOMO}}$ | $\epsilon_{\mathrm{LUMO}}$ | $\mu$-QM9 | $C_v$ | $\mu$-QMe14S |
|---|---|---|---|---|---|---|---|
| Vanilla | **1.570** | 1.538 | 1.538 | 1.514 | 1.526 | 1.550 | 1.698 |
| CFG | **1.570** | 1.540 | 1.545 | **1.551** | **1.557** | **1.577** | **1.770** |
| AG | 1.568 | **1.551** | **1.569** | 1.524 | 1.545 | 1.569 | 1.730 |
| MG | 1.510 | 1.533 | 1.509 | 1.523 | 1.530 | 1.523 | 1.709 |

#### S-5.6.3 Scaffold diversity

**Table S12:** Scaffold diversity of generated molecules under various guidance methods. The highest values are in **bold**, and the second highest values are underlined.

| Property | $\alpha$ | $\Delta\epsilon$ | $\epsilon_{\mathrm{HOMO}}$ | $\epsilon_{\mathrm{LUMO}}$ | $\mu$-QM9 | $C_v$ | $\mu$-QMe14S |
|---|---|---|---|---|---|---|---|
| Vanilla | 0.272 | **0.325** | **0.330** | 0.305 | **0.496** | 0.279 | 0.216 |
| CFG | 0.284 | 0.314 | 0.317 | 0.310 | 0.403 | **0.331** | **0.309** |
| AG | 0.247 | 0.294 | 0.289 | 0.302 | 0.270 | 0.281 | 0.228 |
| MG | **0.369** | 0.242 | 0.328 | **0.354** | 0.331 | 0.277 | 0.281 |

### S-5.7 Training time cost

Table S13 reports the training and sampling wall-clock time for each guidance method. Both training and sampling used one NVIDIA A100 GPU with 80GB memory. Because AG uses the PMF-vanilla's model as its main model, its total training time for the main model along is unchanged. In practice, one needs to either save a checkpoint model with fewer training epochs as the guide model or to train model with less complex architecture (for example, fewer node and edge features), which only takes a negligible additional 2 hours. CFG slightly reduces training time by skipping the property-embedding MLP operations on 10% of the data for the unconditional model. MG incurs a modest training overhead relative to PMF-Vanilla because it maintains an EMA copy of the online model. The MG model thus requires two forwards to obtain its unconditional and conditional predictions to compile the updated training objective (Eq. 10Model Guidanceequation.0.10) without gradient computation, and the EMA copy is updated every training step. The discussion

for sampling efficiency can be found in Figure 5Performance in molecule stability, RDKit validity and uniqueness, sampling efficiency and overall performance for models trained on the rQM9 data. (a) Molecule stability of guidance methods against three baseline conditional models. (b) RDKit validity and uniqueness ratio across our guidance methods. (c) Sampling efficiency across different guidance methods. (d) Overall performance in four dimensions. Results in (a), (b), (c) are reported as the mean ± std across six molecular propertiesfigure.5.

**Table S13:** Training and sampling times. Training is for 2000 epochs and sampling is for 10 k molecules. Values are reported as mean ± standard deviation across the six properties.

| Model | Training [h] ↓ | Sampling [min] ↓ |
|---|---|---|
| Vanilla | 55.4 ± 0.7 | 9.6 ± 0.5 |
| CFG | 54.9 ± 0.5 | 16.8 ± 0.4 |
| AG | 57.4 ± 0.7 | 12.4 ± 1.3 |
| MG | 90.3 ± 3.2 | 9.1 ± 0.5 |

## S-5.8 Ablations

**Guidance weights.** Figure S4 shows how molecule stability varies with guidance weights. For both AG and CFG, increasing the weight on atomic positions ($w_1$) while decreasing the weight on discrete variables ($w_2$) enhances molecule stability. However, AG is far more sensitive to changes in $w_2$ than CFG: AG's molecule stability plummets from over 0.9 at $w_2 = 1$ to about 0.1 at $w_2 = 3$, whereas CFG experiences a much smaller drop ($\leq$ 0.15). This suggests that CFG models are more robust to choices of discrete-variable weights, likely because CFG uses a single network with alternate property embeddings for unconditional and conditional generation, while AG relies on two more loosely coupled networks whose logits of discrete-variable predictions may not be compatible when interpolated with large weights.

The guidance-weight variation for property alignment closely mirror the trends observed in our Bayesian optimization experiments (see Figure S5). Nevertheless, MG models exhibit almost no dependence of molecule stability, bond entropy and property alignment on guidance weights ( Table S16), suggesting that MG struggles to leverage the guidance scaling effects—a phenomenon that merits further investigation.

**Inference timesteps for CFG.** For a good balance between sampling efficiency and accuracy, we use 100 integration timesteps to generate molecules. Table S14 reports the property MAEs for CFG inference with varying numbers of time steps ($n_{\text{ts}}$). Raising $n_{\text{ts}}$ to 200 causes all MAEs to be lower than those of JODO (Table S4). Further increasing $n_{\text{ts}}$ improves the alignment for $\Delta\epsilon$, $\epsilon_{\text{HOMO}}$, and $\epsilon_{\text{LUMO}}$, but has negligible impact on other properties.

**Guidance on all four molecular modalities.** Table S15 compares the property MAEs for CFG using Bayesian-optimized guidance weights across all four modalities, namely atom types, formal charges, bond orders and atom coordinates. The results show that using four separate guidance weights yields performance comparable to using just two: one for positions and one shared across all discrete variables. Similar results are observed for AG (Table S17).

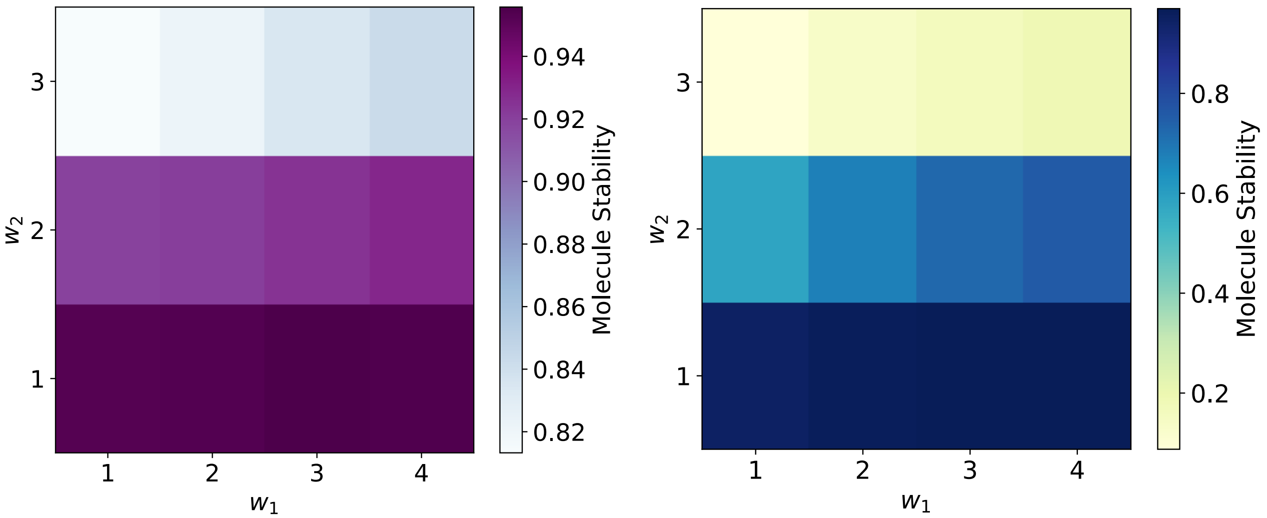


**Figure S4:** Dependence of molecule stability on guidance weights for CFG (Left) and AG (Right). Values are reported by averaging across six properties.

**Table S14:** MAEs for CFG with optimized guidance weights across varying integration timesteps ($n_{\text{ts}}$). Best results are bolded.

| $n_{\text{ts}}$ | $\alpha$ | $\Delta\epsilon$ | $\epsilon_{\text{HOMO}}$ | $\epsilon_{\text{LUMO}}$ | $\mu$-QM9 | $C_v$ | $\mu$-QMe14S |
|---|---|---|---|---|---|---|---|
| 100 | 1.27 | 322 | 220 | 265 | 0.580 | 0.581 | 0.557 |
| 200 | 1.24 | 317 | 222 | 252 | **0.552** | **0.568** | 0.541 |
| 300 | **1.22** | 313 | 219 | 248 | 0.559 | 0.573 | 0.533 |
| 400 | 1.22 | 311 | 219 | 253 | 0.564 | 0.575 | 0.541 |
| 500 | 1.23 | **309** | **215** | **246** | 0.559 | 0.574 | **0.532** |

**Table S15:** Comparison of property MAEs with four guidance weights against two guidance weights for CFG.

| CFG | $\alpha$ | $\Delta\epsilon$ | $\epsilon_{\text{HOMO}}$ | $\epsilon_{\text{LUMO}}$ | $\mu$-QM9 | $C_v$ | $\mu$-QMe14S |
|---|---|---|---|---|---|---|---|
| Two weights | 1.27 | 322 | 220 | 265 | 0.580 | 0.581 | 0.557 |
| Four weights | 1.25 | 343 | 219 | 270 | 0.571 | 0.591 | 0.552 |

Figure S5 shows the property alignment as a function of guidance weights $w_1$ and $w_2$. The guidance weights for the lowest MAE of CFG $\epsilon_{\text{HOMO}}$ are $(w_1, w_2) = (4, 2)$ with a property MAE of 216 meV, and the second lowest MAE comes with $(w_1, w_2) = (3, 2)$ with a MAE of 221 meV, which confirms the findings of the Bayesian analysis. The guidance weights for the lowest MAE of AG $C_v$ are $(w_1, w_2) = (3, 1)$ with an MAE of 0.654 cal/(mol·K), which is slightly worse than the result (0.638 cal/(mol·K)) using the Bayesian-optimized guidance weights $(w_1, w_2) = (2.75, 1.14)$.

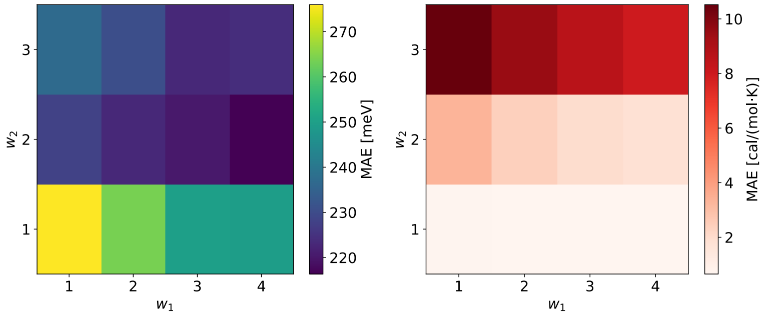


**Figure S5:** Effects of guidance weights on the property alignment for CFG $\epsilon_{\text{HOMO}}$(Left) and AG $C_v$(Right).

Ablation study on the dependence of molecule stability on guidance weights for MG can be found in Table S16.

**Table S16:** Molecule Stability for MG versus guidance weights. This molecule stability and bond distance std is averaged across models conditioned on six properties.

| $w$ | Molecule Stability [%] | Bond Entropy | MAE, $\Delta\epsilon$[meV] |
|---|---|---|---|
| 1 | 95.1 ± 2.1 | 0.536 ± 0.044 | 429 |
| 2 | 95.0 ± 2.1 | 0.535 ± 0.044 | 427 |
| 3 | 95.1 ± 2.3 | 0.533 ± 0.044 | 429 |
| 4 | 95.1 ± 2.1 | 0.536 ± 0.048 | 429 |

Results for guidance on four weights versus guidance on two weights for AG can be found in Table S17.

**Table S17:** Comparison of property MAEs with four guidance weights against two guidance weights for AG.

| AG | $\alpha$ | $\Delta\epsilon$ | $\epsilon_{\text{HOMO}}$ | $\epsilon_{\text{LUMO}}$ | $\mu$-QM9 | $C_v$ | $\mu$-QMe14S |
|---|---|---|---|---|---|---|---|
| Two weights | 1.43 | 344 | 242 | 274 | 0.631 | 0.638 | 0.595 |
| Four weights | 1.46 | 341 | 247 | 265 | 0.620 | 0.640 | 0.584 |

# S-6 Original QM9 Properties and Data Details

Exact definitions for all six molecular properties of QM9 data are shown below.

- $\alpha$ (Polarizability): Tendency of a molecule to acquire an eletric dipole moment when subjected to an external electric field.

- $\Delta\epsilon$: The energy gap between HOMO and LUMO.
- $\epsilon_{\mathrm{HOMO}}$: Highest occupied molecule orbital energy.
- $\epsilon_{\mathrm{LUMO}}$: Lowest unoccupied molecule orbital energy.
- $\mu$: Dipole moment, which measures the separation of positive and negative charges within a molecule.
- $C_v$: Heat capacity at room temperature $298.15$ K.

QM9 is a 134k small molecule dataset that only contains of up to 9 heavy atoms (C, N, O, F). The atom sizes range from 3 to 29 with an average of 18 atoms, including explicit hydrogen. All molecules are optimized by density functional theory (DFT) calculations and thus in their stable states. By design, all molecules in QM9 are charge neural and have a close shell valence electron configuration. But one should note there are molecules that carry explicit atom formal charges and a molecule graph carrying this information might be hence helpful—like we did in this work—to generate molecules with valid charge–valency configuration.

# References


[1] Andrew Campbell, Jason Yim, Regina Barzilay, Tom Rainforth, and Tommi Jaakkola. Generative flows on discrete state-spaces: Enabling multimodal flows with applications to protein co-design. In *Forty-first International Conference on Machine Learning*, 2024.

[2] Ian Dunn and David R. Koes. Exploring discrete flow matching for 3d de novo molecule generation. *arXiv* preprint arXiv:2411.16644, 2024.

[3] Cheng Zeng, Jirui Jin, George Karypis, Mark Transtrum, Ellad B. Tadmor, Richard G. Hennig, Adrian Roitberg, Stefano Martiniani, and Mingjie Liu. Propmolflow: Property-guided molecule generation with geometry-complete flow matching. *arXiv preprint arXiv:2505.21469*, 2025.

[4] Ian Dunn and David Ryan Koes. Mixed continuous and categorical flow matching for 3d de novo molecule generation. *CoRR*, abs/2404.19739, 2024.

[5] Jimmy Lei Ba, Jamie Ryan Kiros, and Geoffrey E. Hinton. Layer Normalization, July 2016.

[6] Alexander Tong, Kilian Fatras, Nikolay Malkin, Guillaume Huguet, Yanlei Zhang, Jarrid Rector-Brooks, Guy Wolf, and Yoshua Bengio. Improving and generalizing flow-based generative models with minibatch optimal transport, March 2024.

[7] Yuxuan Song, Jingjing Gong, Minkai Xu, Ziyao Cao, Yanyan Lan, Stefano Ermon, Hao Zhou, and Wei-Ying Ma. Equivariant Flow Matching with Hybrid Probability Transport for 3D Molecule Generation. *Advances in Neural Information Processing Systems*, 36:549–568, December 2023.

[8] Leon Klein, Andreas Krämer, and Frank Noé. Equivariant flow matching, November 2023.

[9] Emiel Hoogeboom, Vıctor Garcia Satorras, Clément Vignac, and Max Welling. Equivariant Diffusion for Molecule Generation in 3D. In *Proceedings of the 39th International Conference on Machine Learning*, pages 8867–8887. PMLR, June 2022.

[10] Raghunathan Ramakrishnan, Pavlo O Dral, Matthias Rupp, and O Anatole Von Lilienfeld. Quantum chemistry structures and properties of 134 kilo molecules. *Scientific data*, 1(1):1–7, 2014.
